# Supplementary material for: Towards Real-world Event-guided Low-light Video Enhancement and Deblurring
Source: arXiv:2408.14916 source file (2024-08-27)

(a) Low-light blur image

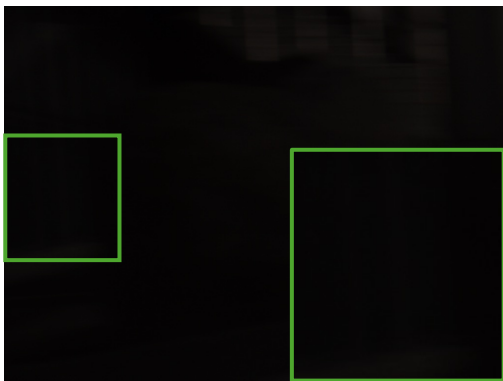

(b) Low-light events

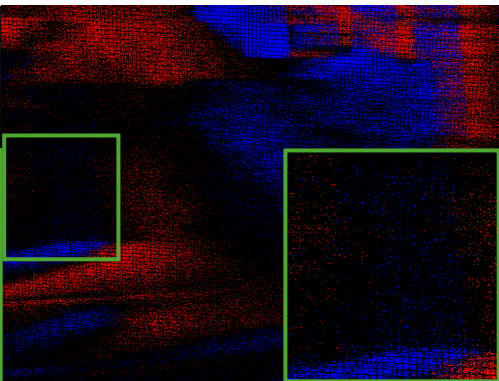

(c) LLFormer

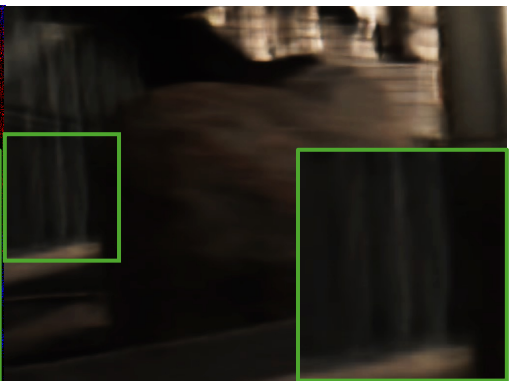

(d) SNRNet

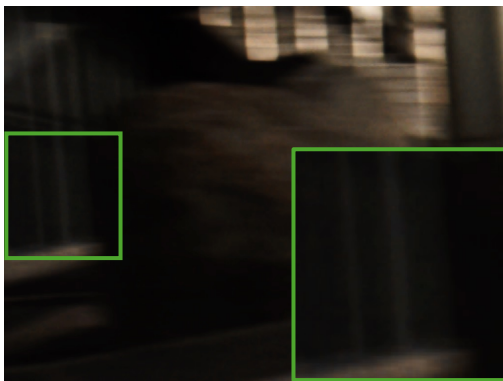

(e) NAFNet

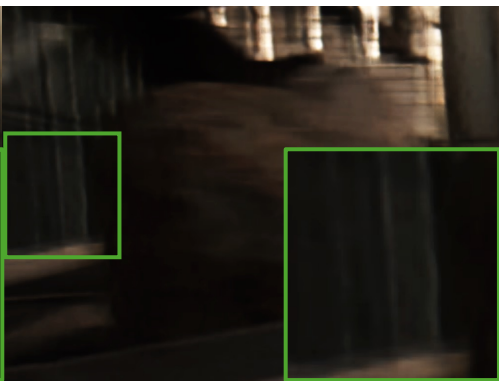

(f) GEM

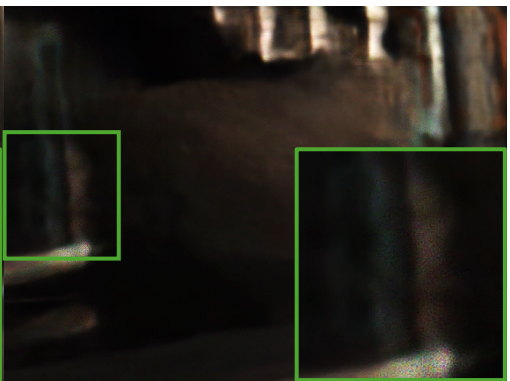

(g) UEVD

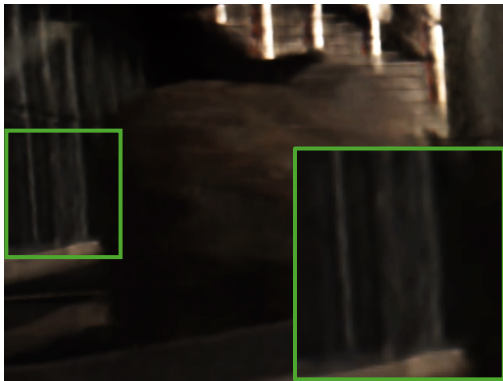

(h) Ours

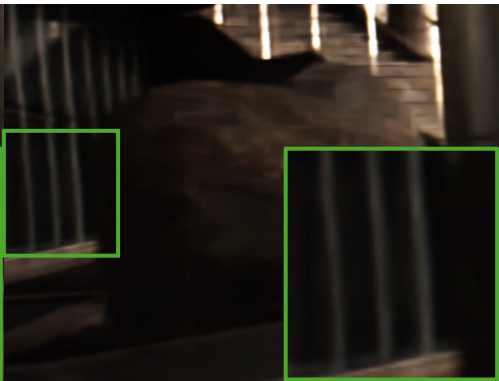

(i) GT

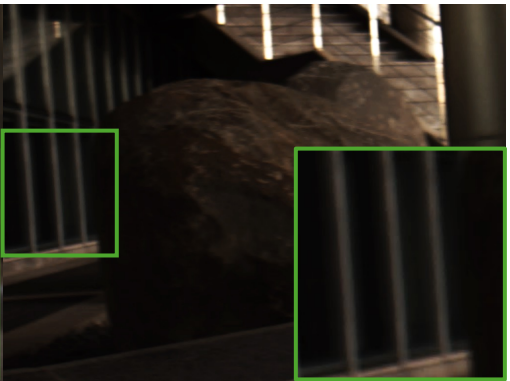

(a) Low-light blur images

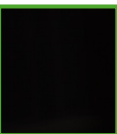

(b) Low-light event

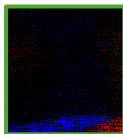

(c) LLFormer

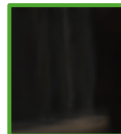

(d) SNRNet

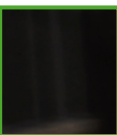

(e) NAFNet

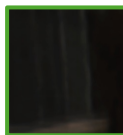

(f) GEM

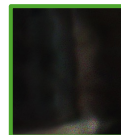

(g) UEVD

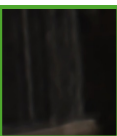

(h) Ours

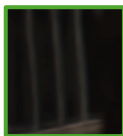

(I) GT

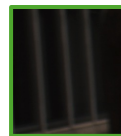

Supplement: Supplementary file 2 [file qual_results_supp_v3.pdf]
